# Supplementary material for: The ParClusterers Benchmark Suite (PCBS): A Fine-Grained Analysis of Scalable Graph Clustering
Source: arXiv:2411.10290 source file (2024-11-15)
Supplement: Supplementary file 1 [file appendic-xc-exp.tex]

\section{Classification with a Large Number of Classes}

\julian{discuss the experiment setup}\shangdi{@Kuba, thanks}

On classification with large number of clusters, we observe that the connectivity algorithm produces the best quality clusters.\laxman{perhaps surprisingly? maybe we can say why once we do a deeper evaluation}

\subsection{Data Set}

\Cref{table:xc_datasets} also contains weighted $k$-nearest neighbor graphs derived from real-world embedding datasets~\cite{Bhatia16}, but here the number of ground truth clusters is much larger than the previous set of datasets. Again, we present the results for $k=50$ here and for $k=10$ and $k=100$ in \Cref{sec:compare_k}. We embed the text using Google Vertex AI's "textembedding-gecko@003" model\footnote{\url{https://cloud.google.com/vertex-ai/generative-ai/docs/embeddings/get-text-embeddings}} with task type "CLUSTERING", where the embeddings all have a dimension of 768. We also tried  OpenAI's "text-embedding-3-small" model where the embeddings all have a dimension of 1536, and observe similar results.
We truncate the text if necessary when they exceed the maximum context length.
The edge weights are cosine similarities on the normalized embeddings. 
The ground truth clusters may be overlapping. We remove duplicate communities in the ground truth (e.g., singleton communities with the same node).

\begin{table}[t]
\small
\centering
\begin{tabular}{|l|l|l|l|}
\hline
\textbf{Dataset} & \textbf{Num. Vertices} & \textbf{Num. Cluster} & \textbf{$\hat{C}$}  \\
\hline
AmazonTitles (AMT) & 636,051 & 569,402 & 5.387  \\
\hline
Amazon (AM2) & 643,474&   571,123 & 5.385 \\
\hline
WikiTitles (WT) & 2,422,400 & 499,081 & 4.775\\
\hline
WikiSeeAlsoTitles (WSAT) &791,909&   331,262 &  2.329\\
\hline
\end{tabular}
\caption{Description of the weighted datasets where the number of ground truth clusters is large compared to the number of vertices. "Num. Cluster" is the number of ground truth clusters and $\hat{C}$ is the average number of clusters that each point belongs to.}
\label{table:xc_datasets}
\end{table}

We show Pareto frontier plots of weighted graphs with a large number of ground truth clusters in \Cref{fig:pr_xc} and the area under the precision-recall curve in \Cref{tab:xc}. Here we do not present the $F_{0.5}$ score because when the number of ground truth clusters are too large and heavily overlapping, this measure is not suitable and the best $F_{0.5}$ score is achieved when all points are in their own singleton cluster.

The result in this regime is quite different from the previous two settings. We see that connectivity is the best method and TECTONIC is the second best. \laxman{It's surprising that TECTONIC (unweighted) works well here.} In terms of running time, similar to previous results, LDD and connectivity are the fastest.

\julian{mention correlation and modularity. say all of them have reasonable quality but worse than TECTONIC and connectivity}
ParHAC with a small approximation parameter has a similar performance to affinity clustering, but ParHAC with a large approximation parameter ($\epsilon=1$) performs very poorly.

LP, SLPA, and SCAN are not suitable for this task because they are not able to produce a very large number of clusters on these datasets. 

We also notice that when the number of clusters is large, choosing a smaller $k$ (e.g., $k=10$) does not change the clustering result much, but when the number of clusters is small, a smaller $k$ makes quality worse. This is because when the number of clusters is large (and the cluster size is small), only very local information is needed for clustering, and so a large $k$ is less beneficial. More details are presented in \Cref{sec:compare_k}.\kuba{Do the algorithms become noticeably faster with smaller $k$?}\shangdi{yes.}
\shangdi{include a boxplot of running times.}

Overall, we recommend that when the number of clusters is large and the size of the clusters is very small, a smaller $k$ can be used when constructing the $k$-nearest neighbor graphs, and the connectivity algorithm is recommended for clustering.

\begin{table}[t]
    \centering
\begin{tabular}{l|ccccc}
\toprule
Clusterer  & AMT & WSAT & AM2 & WT & Mean \\
\midrule
Connectivity & 0.21 & \textbf{ 0.22 } & 0.23  & \textbf{ 0.12 } & \textbf{ 0.19 } \\
TECTONIC &  0.21  & 0.22 & 0.22 & 0.11 & 0.19 \\
Correlation & \textbf{ 0.21 } & 0.22 & \textbf{ 0.23 } & 0.10 & 0.19 \\
ParHac-0.01 & 0.20 & 0.21 & 0.22 & 0.10 & 0.18 \\
ParHac-0.1 & 0.20 & 0.21 & 0.22 & 0.10 & 0.18 \\
Affinity & 0.19 & 0.21 & 0.19 & 0.10 & 0.17 \\
ParHac-1 & 0.16 & 0.19 & 0.16 & 0.09 & 0.15 \\
Modularity & 0.15 & 0.19 & 0.15 & 0.10 & 0.15 \\
LDD & 0.15 & 0.18 & 0.15 & 0.08 & 0.14 \\
Scan & 0.00 & 0.00 & 0.00 & 0.00 & 0.00 \\
LP & 0.00 & 0.00 & 0.00 & 0.00 & 0.00 \\
SLPA & 0.00 & 0.00 & 0.00 & 0.00 & 0.00 \\
\bottomrule
\end{tabular}

    \caption{Area under curve for precision $\geq$ 0.5 on weighted $k$-nearest neighbor graphs with $k=50$.}
    \label{tab:xc}
\end{table}

\begin{figure*}
    \centering
    \includegraphics[width=\textwidth]{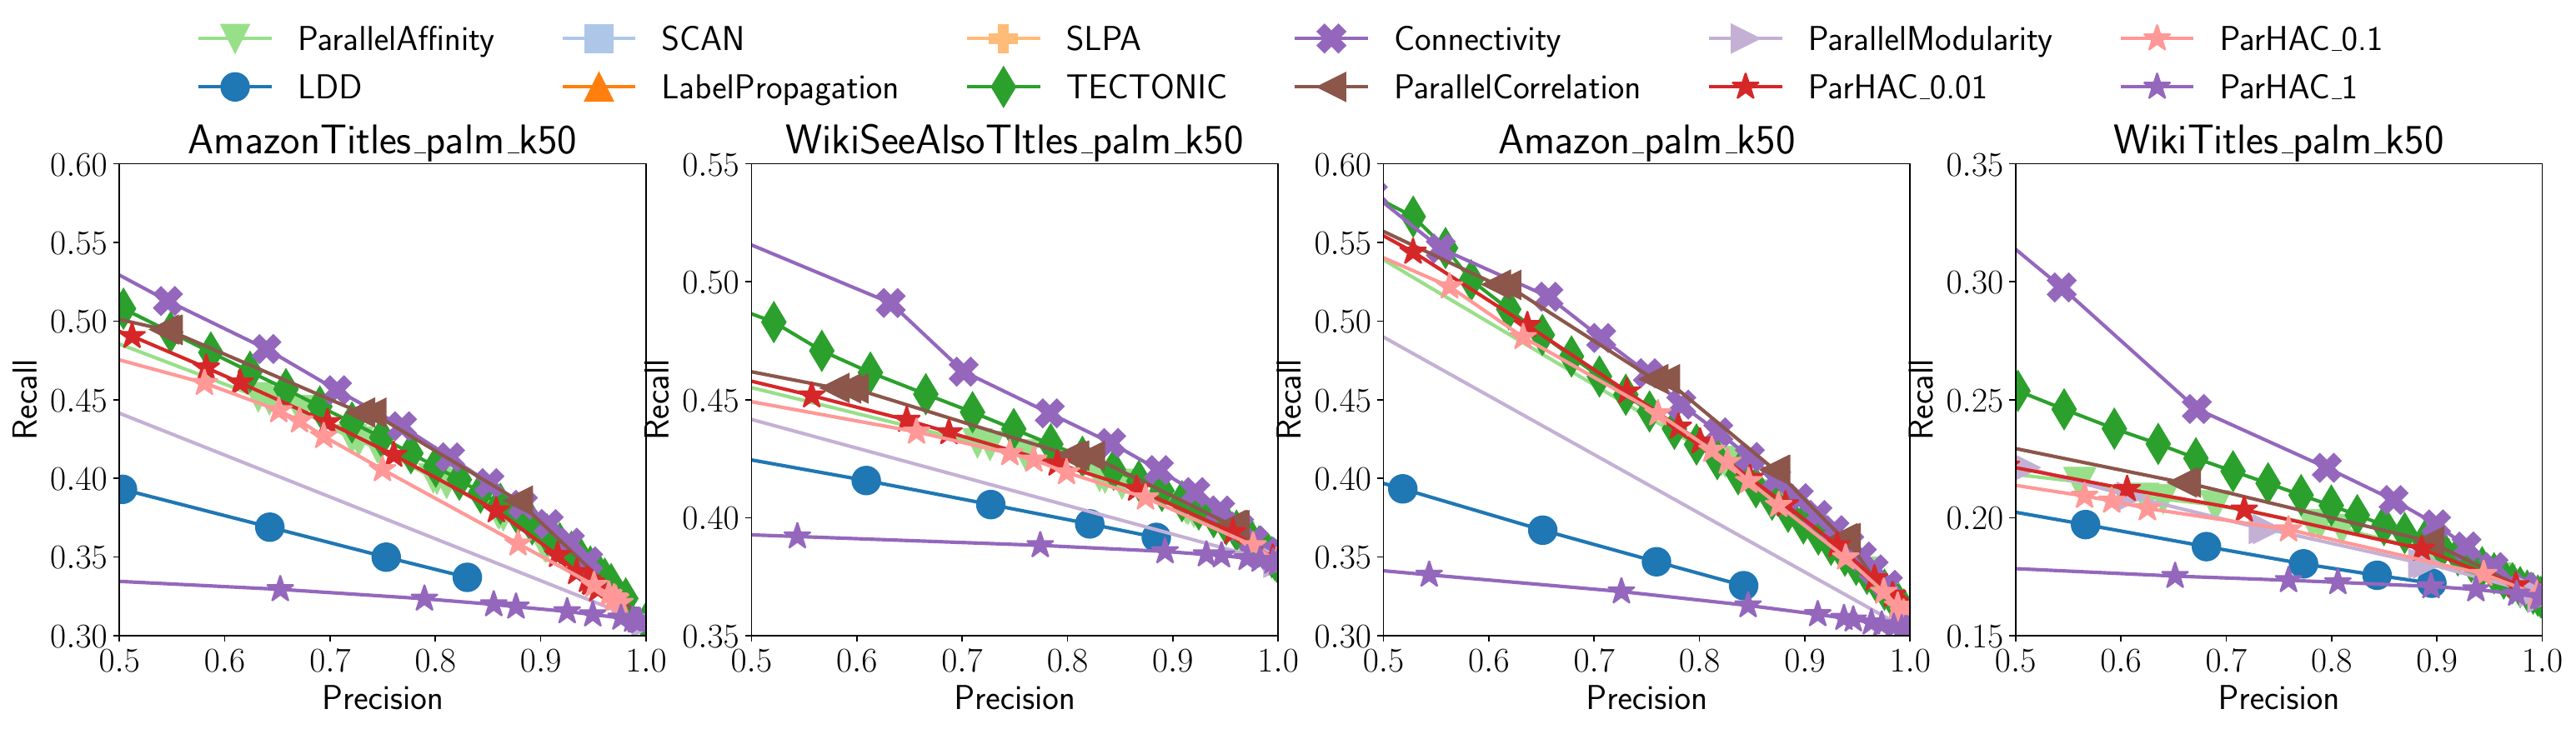}
    \caption{The Pareto frontier of the precision and recall for the weighted XC graphs ($k=50$), using ParClusterer methods. The Pareto frontier of $F_{0.5}$ score and cluster time on \knn graphs with $k=50$. \shangdi{remove palm in titles.}}
    \label{fig:pr_xc}
\end{figure*}
